# Supplementary material for: Parameterized Quantum Query Algorithms for Graph Problems
Source: arXiv:2408.03864 source file (2024-08-07)
Supplement: Supplementary file 1 [file appendix_algorithm_list_model.tex]

\section{Quantum Query Algorithm in the List Model} \label{appendix:quantum_kernelization_list_model}

In this section, we present our quantum kernelization algorithm for the {\sc $k$-vertex cover} problem in the list model.

In the adjacency list model\footnote{There is another model that deals with the adjacency list in the quantum query model\tatsuyadel{, which is called adjacency array model}; see \cite{durr2006quantum}.}, the input graph is given by an array of size $n(n - 1)$ that can be considered as a matrix $L$ of size $n \times (n - 1)$. The $i$--th row of this matrix is a list of neighbors of the $i$--th vertex $v_i$ of the graph $G$. Suppose $v_i$ has degree $d_i$. Then the first $d_i$ coordinates of $i$--th row are filled by the neighbors of $v_i$ in some order, and the last $n - 1 - d_i$ coordinates are filled by a null symbol. Here $L_{i j}$ denotes the $j$--th neighbor of the vertex $v_i$.
In the adjacency list model, a query oracle transformation $O_L$ acts as
$O_L \ket{i, j} \ket{q} = \ket{i, j} \ket{q \oplus L_{ij}}$, where $q \in \{0, \ldots, n\}$ and $\oplus$ denotes addition modulo $n + 1$.

We show the following theorem.
% We show the following theorem, which implies Theorem \ref{thm:main_theorem_list_model}.

\begin{theorem} \label{thm:quantum_query_best_algorithm_vertex_cover_list_model}
Given an integer $k$ and a graph $G$ with n vertices,
there is a bounded error quantum kernelization algorithm for the {\sc $k$-vertex cover} problem using $O(\sqrt{k(m + n)} + k^2)$ queries in the adjacency list model.
\end{theorem}

For the proof, we first show the following lemma
by using the guessing tree method \cite{beigi2020quantum}:

\begin{lemma} \label{lem:find_k_restricted_maximal_matching_list_model}
Given an integer $k$ and a graph $G$ with n vertices,
there is a bounded error quantum algorithm \texttt{\textup{QuantumThresholdMaximalMatchingListModel}} to find a maximal matching of size at most $k$ or conclude that there exists a matching of size at least $k + 1$,
in $O(\sqrt{k(m + n)})$ queries in the adjacency list model.
\end{lemma}

\begin{proof}
In order to apply Theorem \ref{thm:guessing_tree_algorithm}, we first present the following simple classical query algorithm.
We query the $i$-th vertex adjacent to the vertex $v$ one by one until we find a edge whose endpoints do not belong a set of endpoints of the current matching.
If we found such an edge, we add it to the current matching.
If we find a matching of size more than $k$, then we terminate the algorithm and return the matching.
If we see all edges in $G$, we output the current matching.
Here, the depth of the decision tree is $T \leq m + n$.
Note that, since we do not know the degrees of vertices, we stop querying neighbors of each vertex after seeing a null symbol.

Let $W(v, i)$ denote the set of vertices that was added to the current matching
before querying $(v, i)$.
Then, all edges that leave from the vertex corresponding to the query $(v, i)$ and 
correspond to a vertex in $W(v, i)$ or a null symbol
can be grouped into a single edge $e(v, i)$ in the decision tree.
Recall that each internal vertex represents a query, and each outgoing edge from a vertex represents a possible outcome of the query.
In our guessing scheme, we label a edge $e(v, i)$ from each vertex corresponding to a query $(v, i)$ as the guess.

The algorithm returns a matching with at most $k$ edges, or concludes that there exists a matching with at least $k + 1$ edges.
Then, we make at most $I = k + 1$ mistakes.
Recall that the quantity $I$ is the maximum number of incorrect guess in any path from the root to a leaf of the decision tree.
Therefore,
Theorem \ref{thm:guessing_tree_algorithm} implies that the quantum query complexity of solving the $k$-threshold maximal matching problem is $O(\sqrt{TI}) = O(\sqrt{k(m + n)})$,
which completes the proof.
\end{proof}

\begin{algorithm}[H]
    \KwInput{An unweighted graph $G$ in the adjacency list model, an integer $k$}
    \KwOutput{Find a vertex cover of size at most $k$, or conclude that the input graph $G$ does not contain a vertex cover of size at most $k$}
    $M \gets$ \texttt{QuantumThresholdMaximalMatchingListModel}($G, k$) \label{line:quantum_kernelization_list_1} \\
    \If{$|M| > k$} {
        % \tcp{There exists a matching of size at least $k + 1$ in $G$.}
        % \Return Conclude the input instance is a no-instance.
        \Return Conclude the input graph $G$ does not contain a vertex cover of size at most $k$.
    }
    % \If{$2 |M| \leq k$} {
    %     % \Return Conclude the input instance is a yes-instance.
    %     \tcp{We conclude that the input graph $G$ contains a vertex cover of size at most $k$.}
    %     % \Return Conclude the input instance is a yes-instance.
    %     \Return The vertex set $V(M)$ is a vertex cover in $G$.
    % }
    % $G' \gets G$ \\
    $U \gets \emptyset$, $E' \gets \emptyset$, $k' \gets k$ \\
    For $v \in V(M)$, $N_v \gets \emptyset$ \\
    \For{$v \in V(E_M)$} { \tcp{Denote by $V(E_M)$ the set of endpoints of edges in $E_M$}
        % \If{\texttt{\textup{Query}}$(v, k + 1) \neq \text{\textup{null}}$} {
        %     $U \gets U \cup \{v\}$ \\
        %     $k' \gets k' - 1$
        % } 
        % $N_v \gets \emptyset$ \label{line:quantum_kernelization_list_2} \\
        \For{$i \leftarrow 1 $ \KwTo $k + 1$} { 
            $w \gets$ \texttt{Query}$(v, i)$ \label{line:quantum_kernelization_list_2} \\
            \If{$w =$ \textup{null}} {
                \Break
            }
            \If{$w \notin U$} {
                $N_v \gets N_v \cup \{w\}$
            }
        }
        \If{$|N_v| \leq k'$} {
            \For{$w \in N_v$} {
                $E' \gets E' \cup \{(v, w)\}$ \\
            }
        } \Else {
            $U \gets U \cup \{v\}$ \\
            $k' \gets k' - 1$
        }
    }   
    $G' \gets (V(E'), E')$ \\
    \tcp{Denote by $V(E')$ a set of endpoints of edges in $E'$}
    % \Return $(G', k')$ 
    Solve the {\sc $k$-vertex cover} problem for the instance $(G',  k')$ by a known classical algorithm.  \\
    % \Return $(G', k')$ 
    \If{The classical algorithm finds a vertex cover $S$ in $G'$} {
        \Return The vertex set $S \cup U$ is a vertex cover in $G$.
    } \Else {
        \Return Conclude the input graph $G$ does not contain a vertex cover of size at most $k$.
    }
    \caption{\texttt{Quantum $k$-Vertex Cover in the List Model}}\label{alg:quantum_vertex_cover_list}
\end{algorithm}

Now we give a proof of Theorem \ref{thm:quantum_query_best_algorithm_vertex_cover_list_model}.

\begin{proof}[Proof of Threorem \ref{thm:quantum_query_best_algorithm_vertex_cover_list_model}]
The correctness of \texttt{Quantum $k$-Vertex Cover  in the List Model} (Algorithm \ref{alg:quantum_vertex_cover_list}) follows from the correctness of \texttt{Quantum $k$-Vertex Cover} (Algorithm \ref{alg:quantum_vertex_cover}).

Next we analyze the query complexity used in Algorithm \ref{alg:quantum_vertex_cover_list}.
By Lemma \ref{lem:find_k_restricted_maximal_matching_list_model}, 
we use $O(\sqrt{k(m + n)})$ queries in Line \ref{line:quantum_kernelization_list_1}.
Furthermore, since the size of $V(M)$ is at most $2 k$,
% the size of $V(E_M)$ is at most $2 k$.
we use $O(k^2)$ queries in Line \ref{line:quantum_kernelization_list_2},
which completes the proof.
\end{proof}
